# Supplementary material for: Settling the Sample Complexity of Model-Based Offline Reinforcement Learning
Source: arXiv:2204.05275 source file (2024-03-08)
Supplement: Supplementary file 1 [file appendix_lower_bound.tex]

\section{Proof of minimax lower bounds}
\subsection{Proof of Theorem~\ref{thm:finite-lower-bound}}

\paragraph{Preliminary definitions and facts}
\yxc{define KL here}
\paragraph{Construction of the hard MDPs.}
To begin with, consider a collection of MDPs $\mathcal{M}_{\theta} = (\mathcal{S}, \mathcal{A}, P^{\theta} = \{P^{\theta_h}_h\}_{h=1}^H, \{r_h\}_{h=1}^H, H)$ parameterized by $\theta$, 
where $\cS = \{0, 1, \ldots, S-1\}$, $\mathcal{A} = \{0, 1\}$, and $\theta = \{\theta_h\}_{h=1}^H \in \Theta \subseteq \{0, 1\}^{H}$. Suppose that $H\geq 32$ and there exist a constant $C \geq \frac{4}{S}$. We also find it convenient to introduce the following state distribution: \yxc{what is $C$?}
\begin{align}\label{finite-mu-assumption}
       \mu(s) = \frac{1}{CS}\mathds{1}(s = 0) + \Big(1 - \frac{1}{CS}\Big)\mathds{1}(s = 1), \qquad \text{where } \frac{1}{CS} \leq \frac{1}{4}.
\end{align}
With this distribution in hand, we define the transition kernel $P^{\theta}$ of the MDP $\mathcal{M}_\theta$ as follows:
\begin{align*}
P^{\theta_h}_h(s^{\prime} \mymid s, a) = \left\{ \begin{array}{lll}
         p\mathds{1}(s^{\prime} = 0) + (1-p)\mu(s^{\prime}) & \text{if} & (s, a) = (0, \theta_h), \\
         q\mathds{1}(s^{\prime} = 0) + (1-q)\mu(s^{\prime}) & \text{if} & (s, a) = (0, 1-\theta_h), \\
         \mathds{1}(s^{\prime} = s) & \text{if}   & (s, a) = (1, 0), \\ 
         \big(1 - \frac{2}{H}\big)\mathds{1}(s^{\prime} = s) + \frac{2}{H}\mu(s^{\prime}) & \text{if}   & (s, a) = (1, 1), \\ 
         H\mathds{1}(s^{\prime} = s) + \frac{1}{H}\mu(s^{\prime}) & \text{if}   & s > 1, \
                \end{array}\right.
\end{align*}
where $p$ and $q$ are defined to be 
\begin{equation}
	p = 1 - \frac{1}{H} + \frac{c\varepsilon}{H^2}
	\qquad \text{and} \qquad
	q = 1 - \frac{1}{H} - \frac{c\varepsilon}{H^2}
\end{equation}
for some constant $c > 0$ large enough.
In addition, the reward function of these MDPs are taken to be
\begin{align*}
r_h(s, a) = \left\{ \begin{array}{lll}
         1 & \text{if} & s = 0 ,\\
         \frac{1}{2} & \text{if}   & (s, a) = (1, 0), \\ 
         0 & \text{if}   & (s, a) = (1, 1), \\ 
         0 & \text{if}   & s > 1 \text{ and } s\in\cS.\
                \end{array}\right.
\end{align*}

\paragraph{Construction of the batch dataset.}
Correspondingly, we generate a batch dataset with the following initial state distribution $\rhob$ and behavior policy $\pib$: 
\begin{align*}
	\rhob (s) = \mu(s)\quad \text{and } \quad\pi_h^{\mathsf{b}}(a \mymid s) = \frac{1}{2} \qquad \forall (s,a,h)\in \cS\times \cA\times [H], 
\end{align*}
where $\mu$ has been defined in \eqref{finite-mu-assumption}. 
As a result, making use of the definition \eqref{eq:dhb-finite} of $\myrho_h(s, a)$ in and applying a little algebra, one can easily verify that 
\begin{align}
\myrho_h(s) &= d_h^{\pib}(s; \rhob) = \mu(s), \qquad \forall (s,h)\in\cS\times [H],
\end{align}
which directly implies that
\begin{align}
\myrho_h(s, a) &= d_h^{\pib}(s,a; \rhob) =\myrho_h(s)\pi_h^{\mathsf{b}}(a \mymid s) =  \mu(s)\pi_h^{\mathsf{b}}(a \mymid s), \qquad \forall (s,a,h)\in\cS\times \cA\times [H].
\end{align}

With above definitions, now we are ready to derive the lower bound.
\paragraph{Useful facts of hard MDPs.}
We set the goal as learning  a $\varepsilon$-optimal policy with a specific initial state distribution $\rho(s) = \ind(s = 0)$ w.r.t a particular MDP $\mathcal{M}_\theta$, i.e.,
\begin{align}
      \mathcal{L}(\pi, \mathcal{M}_\theta, \rho) =  \big\langle \rho, V_1^{\theta, \star} - V_1^{\pi} \big\rangle \ge \varepsilon.
\end{align}
To begin with, for any policy $\pi$, it is observed that the value of state $s=0$ is
\begin{align}
V_h^{\pi}(0) &= \mathbb{E}_\pi [1 + \gamma P_{s, \pi(s)}V^\pi]\\
& = 1 + \gamma \pi_h(\theta_h \mymid 0) \left[ \big(p + (1-p)\mu(0)\big) V^{\pi}_{h+1}(0) + (1-p) \mu(1) V^{\pi}_{h+1}(1)\right] \nonumber \\
&\qquad + \gamma \pi(1-\theta_h \mymid0) \left[ \big(q + (1-q)\mu(0)\big)V^{\pi}_{h+1}(0) + (1-q)\mu(1) V^{\pi}_{h+1}(1)\right] \nonumber\\
& = 1 + \gamma\left[p \pi_h(\theta_h \mymid 0) + q \pi(1-\theta_h \mymid0) + \mu(0) - p \pi_h(\theta_h \mymid 0) \mu(0) - q \pi(1-\theta_h \mymid0)\mu(0) \right]V^{\pi}_{h+1}(0) \nonumber\\
&\qquad + \gamma \mu(1) \left[ 1 - p\pi_h(\theta_h \mymid 0)  -q \pi(1-\theta_h \mymid 0)\right]V^{\pi}_{h+1}(1) \nonumber\\
& \overset{\mathrm{(i)}}{=} 1 + \gamma \left[ x_h + (1- x_h)\mu(0) V^{\pi}_{h+1}(0) +  (1 - x_h) \mu(1) V^{\pi}_{h+1}(1)\right]  \nonumber\\
& =  1 + \big(\mu(1)x_h+\mu(0)\big) V_{h+1}^{\pi}(0) + (1-x_h)\mu(1)V_{h+1}^{\pi}(1), \label{eq:finite-Value-0}
\end{align}
where (i) holds by letting 
\begin{align}
x_h = p\pi_h(\theta_h\mymid 0) + q\pi_h(1-\theta_h\mymid 0).\label{eq:finite-x-h}
\end{align}
Applying \eqref{eq:finite-Value-0} leads to 
\begin{align}
    V_h^{\pi}(0) = \sum_{h = 1}^H \prod_{j = 1}^{h - 1}\big(\mu(1)x_j+\mu(0)\big)\big[1 + (1-x_h)\mu(1)V_{h+1}^{\pi}(1)\big]. \label{eq:infinite-Value-0-recursive}
\end{align}
Additionally,  the value of state $s=1$ obeys

\begin{align*}
        V_h^{\pi}(1) &= \pi_h(0 \mymid 1) \left( \frac{1}{2} +  V_{h+1}^{\pi}(1)\right) + \pi_h(1 \mymid 1) \left[ \left(1- \frac{2}{HCS}\right)V_{h+1}^{\pi}(1) + \frac{2}{HCS}V_{h+1}^{\pi}(0)\right]\\
        & \overset{\mathrm{(i)}}{\leq} \pi_h(0 \mymid 1) \left( \frac{1}{2} +  V_{h+1}^{\pi}(1)\right) + \pi_h(1 \mymid 1) \left[ \left(1- \frac{2}{HCS}\right)V_{h+1}^{\pi}(1) + \frac{2}{HCS}\left(H -h\right)\right]\\
        & \overset{\mathrm{(ii)}}{\leq} \pi_h(0 \mymid 1) \left( \frac{1}{2} +  V_{h+1}^{\pi}(1)\right) + \pi_h(1 \mymid 1) \left[\frac{1}{2} + \left(1- \frac{2}{HCS}\right)V_{h+1}^{\pi}(1) \right]\\
        & \leq \frac{1}{2} + V_{h+1}^{\pi}(1) - \frac{2}{HCS}\pi_h(1 \mymid 1)
\end{align*}
where (i) arises from the trivial facts $ 0\leq V_h^{\pi}(s) \leq H-h+1$ for any policy $\pi$ and all $(s,h)\in\cS \times [H]$, and (ii) holds from \eqref{finite-mu-assumption}.
The above result implies that the optimal policy $\pi^\star_h(1) = 0$ for all $h\in[H]$ which recursively yields
\begin{align}
        V_h^{\pi}(1) &\le V_h^{\star}(1) = \frac{1}{2}(H+1-h).
\end{align}

To continue, we shall control the term of interest under the condition 
\begin{align}
\|\pi(0) - \pi_\theta^{\star}(0)\|_1 \ge \frac{H}{16}. \label{eq:finite-lower-delta}
\end{align}
Note that it is easily verified that the optimal policy for $\mathcal{M}_\theta$ at state $0$ is $\pi_\theta^\star(0) = \theta = [\pi^\star_1(0), \pi^\star_2(0), \cdots, \pi^\star_H(0)]^\top$, where $\pi^\star_h(0) = \theta_h$ for all $h\in[H]$. \lxs{There are still something need to be specified}As a result, plugging in \eqref{eq:infinite-Value-0-recursive} and $\rho(s) = \ind(s = 0)$,  we arrive at
\begin{align}
    &\langle \rho, V^{\star} - V^{\pi}\rangle = V_1^{\star}(0) - V_1^{\pi}(0) \nonumber \\
    & =  \sum_{h = 1}^H \prod_{j = 1}^{h - 1}\big(\mu(1)p+\mu(0)\big)\big[1 + (1-p)\mu(1)V_{h+1}^{\star}(1)\big] - \sum_{h = 1}^H \prod_{j = 1}^{h - 1}\big(\mu(1)x_j+\mu(0)\big)\big[1 + (1-x_h)\mu(1)V_{h+1}^{\pi}(1)\big] \nonumber \\
    &\ge \sum_{h = 1}^H \prod_{j = 1}^{h - 1}\big(\mu(1)p+\mu(0)\big)\big[1 + (1-p)\mu(1)V_{h+1}^{\star}(1)\big] - \sum_{h = 1}^H \prod_{j = 1}^{h - 1}\big(\mu(1)x_j+\mu(0)\big)\big[1 + (1-x_h)\mu(1)V_{h+1}^{\star}(1)\big] \nonumber \\
     & \overset{\mathrm{(i)}}{\geq} \prod_{h' = 1}^{\left \lfloor \frac{15H}{16}\right \rfloor}\big(\mu(1)p+\mu(0)\big) \sum_{h=\left \lfloor \frac{15H}{16} \right \rfloor}^H \prod_{j = 1}^{h - 1}\big(\mu(1)p+\mu(0)\big)\big[1 + (1-p)\mu(1)V_{h+1}^{\star}(1)\big] \nonumber \\
     &\qquad - \prod_{h' = 1}^{\left \lfloor \frac{15H}{16}\right \rfloor}\big(\mu(1)p+\mu(0)\big)\sum_{h=\left \lfloor \frac{15H}{16} \right \rfloor}^H \prod_{j = 1}^{h - 1}\big(\mu(1)q+\mu(0)\big)\big[1 + (1-q)\mu(1)V_{h+1}^{\star}(1)\big] \nonumber \\
    & = \prod_{h' = 1}^{\left \lfloor \frac{15H}{16}\right \rfloor}\big(\mu(1)p+\mu(0)\big)\underbrace{ \sum_{h=\left \lfloor \frac{15H}{16} \right \rfloor}^H  \left[\prod_{j = 1}^{h - 1}\big(\mu(1)p+\mu(0)\big) - \prod_{j = 1}^{h - 1}\big(\mu(1)q+\mu(0)\big)\right]\big[1 + (1-p)\mu(1)V_{h+1}^{\star}(1)\big]}_{\eqqcolon A} \nonumber \\
    &\qquad - \prod_{h' = 1}^{\left \lfloor \frac{15H}{16}\right \rfloor}\big(\mu(1)p+\mu(0)\big) \underbrace{ \sum_{h=\left \lfloor \frac{15H}{16} \right \rfloor}^H \prod_{j = 1}^{h - 1}\big(\mu(1)q+\mu(0)\big)\big(p-q\big)\mu(1)V_{h+1}^{\star}(1)}_{\eqqcolon B} \nonumber \\
    & = \prod_{h' = 1}^{\left \lfloor \frac{15H}{16}\right \rfloor}\big(\mu(1)p+\mu(0)\big)  \left(A-B\right), \label{eq:finite-A-B}
\end{align}
where (i) arises from the condition \eqref{eq:finite-lower-delta}.

Before continuing, we introduce the following facts which can be easily verified by basic calculus:
\begin{align} \label{eq:basic-facts-finite}
    e^{-\alpha/2} \geq \left(1-\frac{1}{H}\right)^{\alpha H} \geq e^{-\alpha} \geq \frac{1}{e} \quad \text{ and } \left(1-\frac{2}{H}\right)^{\alpha H} \leq e^{-\alpha/4}, \qquad \forall \alpha \in (0,1], H\geq 2.
\end{align}
As a result, we arrive at
\begin{align}
    \prod_{h' = 1}^{\left \lfloor \frac{15H}{16}\right \rfloor}\big(\mu(1)p+\mu(0)\big) =\left(\frac{1}{CS} + \left(1-\frac{1}{CS}\right)\left(1-\frac{1}{H} + \frac{c\varepsilon}{H^2}\right)\right)^{\frac{15H}{16}} \geq \left(1-\frac{1}{H} \right)^{\frac{15H}{16}} \geq \frac{1}{5}.
\end{align}
To control the two terms in \eqref{eq:finite-A-B}, we observe that $B$ can be controlled as
\begin{align}
    \sum_{h=\left \lfloor \frac{15H}{16} \right \rfloor}^H \prod_{j = 1}^{h - 1}\big(\mu(1)q+\mu(0)\big)\big(p-q\big)\mu(1)V_{h+1}^{\star}(1) &\leq  \sum_{h=\left \lfloor \frac{15H}{16} \right \rfloor}^H  \frac{2c\varepsilon}{H^2}V_{h+1}^{\star}(1)= \sum_{h=\left \lfloor \frac{15H}{16} \right \rfloor}^H  \frac{2c\varepsilon}{H^2} \frac{1}{2}(H-h)\\
    & = \frac{c\varepsilon}{H^2} \frac{H}{16}\left(1+\frac{H}{16}\right) \leq \frac{c\varepsilon}{128}, 
\end{align}
where the first inequality holds by $\prod_{j = 1}^{h - 1}\big(\mu(1)q+\mu(0)\big) \leq 1$, $\mu(1) <1$, and the last inequality holds by $1\leq \frac{H}{16}$. For another term $A$, we introduce the following result which shall be verified later
\begin{align} \label{eq:finite-delta-key}
 A \geq c' \varepsilon.
\end{align}

Summing up the results in \eqref{eq:finite-delta-key}, we have 
\begin{align}
 \mathcal{L}(\pi, \mathcal{M}_{\theta}, \rho) = \langle \rho, V^{\theta, \star} - V^{\pi}\rangle = V^{\star}(0) - V^{\pi}(0) \ge \varepsilon
	%, \qquad \forall \pi \in \{\|\pi(0) - \pi_\theta^{\star}(0)\|_1 \ge \frac{H}{16}\}. 
	\label{eq:finite-delta-conclusion}
\end{align}
for any policy $\pi$ obeying $\|\pi(0) - \pi^{\star}(0)\|_1 \ge H/16$.

\paragraph{Deriving the lower bound.}
Applying Gilbert-Varshamov lemma, we can obatain a set $\Theta \subseteq  \{0, 1\}^{H}$ which obeys that $|\Theta| \ge e^{H/8}$ and $\|\theta_i - \theta_k\|_1 \ge \frac{H}{8}$ for any $\theta_i \ne \theta_k \in \Theta$. Note that each $\theta \in \Theta$ uniquely determines a  transition kernel $P^\theta$ and thus a MDP $\mathcal{M}_\theta$. Applying \eqref{eq:finite-delta-conclusion}, we directly arrive at for any policy $\pi$ and $\theta_1 \neq \theta_2$,
\begin{align}
    \mathcal{L}(\pi, \mathcal{M}_{\theta_1}, \rho) + \mathcal{L}(\pi, \mathcal{M}_{\theta_2}, \rho) \geq \epsilon,
\end{align}
since $\|\theta_1 - \theta_2\|_1 \ge H/8$ implies
\begin{align*}
    \sup_{\theta \in \{\theta_1, \theta_2\}} \|\pi(0) - \pi_\theta^{\star}(0)\|_1 &\geq \frac{1}{2} \left(\|\pi(0) - \pi_{\theta_1}^{\star}(0)\|_1 + \|\pi(0) - \pi_{\theta_2}^{\star}(0)\|_1\right)\\
    & = \frac{1}{2} \left(\|\pi(0) - \theta_1\|_1 + \|\pi(0) - \theta_2\|_1\right) \\
    &\geq \frac{1}{2}\|\theta_1 - \theta_2\|_1 \geq \frac{H}{16}.
\end{align*}
% The Gilbert-Varshamov bound tells us there exists $\Theta \subset \{0, 1\}^{H}$ such that $|\Theta| \ge 2^{H/8}$ and $\|\theta_i - \theta_k\|_1 \ge \frac{H}{8}$ for any $\theta_i \ne \theta_k \in \Theta$.

In addition,
\begin{align}
\mathsf{KL}(q \parallel p) &= q\log \frac{q}{p} + (1-q)\log \frac{1-q}{1-p} \nonumber \\
& = q\log \left(1 + \frac{q-p}{p}\right) +(1-q)\log\left(1 + \frac{p-q}{1-p}\right) \nonumber\\
&\leq (q-p)\frac{q}{p} + (p-q)\frac{1-q}{1-p}\\
& = (p-q)\left(\frac{p-q}{p}-1 + 1 + \frac{p-q}{1-p}\right) \nonumber\\
&\leq (p-q)^2 \frac{1}{p(1-p)} \nonumber\\
&\leq \frac{4c^2\varepsilon^2}{H^4} \frac{1}{\left(1-\frac{1}{H} + \frac{c\varepsilon}{H^2}\right) \left(\frac{1}{H} - \frac{c\varepsilon}{H^2}\right)} \nonumber\\
& \leq\frac{16c^2\varepsilon^2}{H^3}, \label{eq:finite-KL-dis}
\end{align}
where the last inequality holds by $\frac{c\varepsilon}{H^2}<\frac{1}{2H}$ and $1-\frac{1}{H} + \frac{c\varepsilon}{H^2} \leq 1-\frac{1}{H} \leq \frac{1}{2}$.
% \begin{align*}
% \mathsf{KL}(p \parallel q) &= p\log \frac{p}{q} + (1-p)\log \frac{1-p}{1-q} \nonumber \\
% & = p\log \left(1 + \frac{p-q}{q}\right)- (1-p)\log\left(1 + \frac{p-q}{1-p}\right) \\
% &\leq (p-q) \frac{p}{q} - (p-q)\\
% & =  \frac{(p-q)^2}{q}\\
% &\leq\frac{4c^2\varepsilon^2}{H^4} \frac{1}{1-\frac{1}{H} - \frac{c\varepsilon}{H^2}}
% \asymp \frac{\varepsilon^2}{H^3}.
% \end{align*}
Now we are ready to apply Fano's inequality, i.e.,
\begin{align}
    \inf_{\pi} \sup_{\mathcal{M}_\theta \mymid \theta\in\Theta} \mathbb{E}[\mathcal{L}(\pi, \mathcal{M}_\theta, \rho)] &\geq \frac{\varepsilon}{2} \left(1-\frac{N \max_{i\neq j} \mathsf{KL}( \mu \bigotimes P^{\theta_i} \parallel \mu \bigotimes P^{\theta_j}) + \log 2 }{\log |\Theta|}\right)\\
    & \overset{\mathrm{(i)}}{\geq} \frac{\varepsilon}{2} \left(1-\frac{N  \cdot \left(\frac{16c^2\varepsilon^2}{H^3} \frac{1}{CS} \right)+ \log 2 }{\log |\Theta|}\right) \\
    &\overset{\mathrm{(ii)}}{\geq} \frac{\varepsilon}{2} \left(1-\frac{N  \frac{128c^2\varepsilon^2}{CSH^3} + \log 2 }{H}\right) \\
    &\overset{\mathrm{(iii)}}{\geq} \frac{\varepsilon}{2} \left(1-\frac{N  \frac{128c^2\varepsilon^2}{CSH^3} + \log 2 }{H}\right) \geq \frac{\varepsilon}{2}\left(1-\frac{1}{3}\right) \geq \frac{\varepsilon}{3},
\end{align}
where (i) arises from \eqref{eq:finite-KL-dis} and $\mu(0) = \frac{1}{CS}$, (ii) holds by $|\Theta| \ge e^{H/8}$, and (iii) follows from
\begin{align}
    N \leq \frac{CSH^4}{768c^2\varepsilon^2}, 
\end{align}
and $\log(2) \leq H/6$.

Hence, 
\begin{align}
     \inf_{\pi} \sup_{\mathcal{M}_\theta \mymid \theta\in\Theta} \mathbb{E}[\mathcal{L}(\pi, \mathcal{M}_\theta, \rho)] \geq \min \left( \frac{1}{3}\sqrt{\frac{CSH^4}{768c^2N}}, H \right)
\end{align}
by setting $\varepsilon = \sqrt{\frac{CSH^4}{768c^2N}}$ if $\frac{1}{3}\sqrt{\frac{CSH^4}{768c^2N}} \leq H$ and $\varepsilon = 3H$ otherwise.
% \begin{align*}
% \inf_{\pi}\sup_{\mathcal{M}_{\theta}} \mathbb{P}\big(\langle \rho, V_1^{\star} - V_1^{\pi}\rangle \ge \varepsilon\big) \ge \frac{1}{3},
% \end{align*}
% since there are $O\left(\frac{H^4}{\varepsilon^2}\right)$ samples for $s = 0$,
% provided that
% \begin{align*}
% N \lesssim \frac{CH^4S}{\varepsilon^2},
% \end{align*}

Notice that for $\pi^{\star}(0) = \theta$, we have 
\begin{align*}
d_h^{\star}(0, \theta) \ge \rho(0)\prod_{j = 1}^{h-1}P_{j}(0 \mymid 0, \theta) \ge \big(1-\frac{1}{H}\big)^{h-1}\rho(0) \ge \frac{1}{e}.
\end{align*}
Plugging in the definition of $\Cstar$, we have 
\begin{align}
    \Cstar  = \max_{(s, a, h) \in \cS \times \cA \times [H]}\frac{\min\big\{d_h^{\star}(s, a), \frac{1}{S}\big\}}{\myrho_h(s, a)} = \max_{h} \frac{\min\big\{d_h^{\star}(0, \theta), \frac{1}{S}\big\}}{\myrho_h(0, \theta)} = \frac{2}{S\mu(0)} = 2C.
\end{align}
As a result, we complete the proof by replacing $C$ by $\Cstar$
\begin{align}
     \inf_{\pi} \sup_{\mathcal{M}_\theta \mymid \theta\in\Theta} \mathbb{E}[\mathcal{L}(\pi, \mathcal{M}_\theta, \rho)] \geq \min \left( \frac{1}{3}\sqrt{\frac{\Cstar SH^4}{768c^2N}}, H \right),
\end{align}
which yields
\begin{align}
    \inf_{\pi} \sup_{\mathcal{M}_\theta \mymid \theta\in\Theta} \mathbb{E}[\mathcal{L}(\pi, \mathcal{M}_\theta, \rho)] \geq \varepsilon
\end{align}
when 
\begin{align}
 N\leq \frac{1}{3}\frac{\Cstar SH^4}{768c^2\varepsilon^2} \leq \frac{c_1 \Cstar SH^4}{\varepsilon^2}.
\end{align}
% Hence, one can check that $\Cstar = \frac{2}{S\mu(0)} = 2C$, and the lower bound is ready.

\paragraph{Proof of \eqref{eq:finite-delta-key}.}
To begin, we observe that
\begin{align}
    A &\overset{\mathrm{(i)}}{\geq} \sum_{h=\left \lfloor \frac{15H}{16} \right \rfloor}^H  \left(\prod_{j = 1}^{h - 1}\big(\mu(1)p+\mu(0)\big) - \prod_{j = 1}^{h - 1}\big(\mu(1)q+\mu(0)\big)\right)  \nonumber \\
    & \geq \frac{1-\big(\mu(1)p+\mu(0)\big)^{H/16}}{1- \big(\mu(1)p+\mu(0)\big)} - \frac{1-\big(\mu(1)q+\mu(0)\big)^{H/16}}{1- \big(\mu(1)q+\mu(0)\big)} \nonumber\\
    & = \frac{(p-q) + (1-p)\big(\mu(1)q+\mu(0)\big)^{H/16} - (1-q)\big(\mu(1)p+\mu(0)\big)^{H/16}}{\mu(1) (1-p)(1-q)} \nonumber \\
&= \frac{ (p-q) + (1-p)\left[\big(\mu(1)q+\mu(0)\big)^{H/16} - \big(\mu(1)p+\mu(0)\big)^{H/16} \right] + (q-p)\big(\mu(1)p+\mu(0)\big)^{H/16}}{\mu(1) (1-p)(1-q)} \nonumber \\
    & =\frac{(p-q) \left(1-\big(\mu(1)p+\mu(0)\big)^{H/16}\right)}{\mu(1) (1-p)(1-q)} - (1-p)\frac{ \big(\mu(1)p+\mu(0)\big)^{H/16} - \big(\mu(1)q+\mu(0)\big)^{H/16}  }{\mu(1) (1-p)(1-q)} \nonumber \\
  & \overset{\mathrm{(ii)}}{\geq}  \frac{\frac{2c\varepsilon}{H^2}(1-e^{-\frac{1}{32}})}{\mu(1) (1-p)(1-q)}- (1-p)\frac{ \big(\mu(1)p+\mu(0)\big)^{H/16} - \big(\mu(1)q+\mu(0)\big)^{H/16}  }{\mu(1) (1-p)(1-q)} \nonumber\\
  & \geq \frac{\frac{0.06 c\varepsilon}{H^2}}{\mu(1) (1-p)(1-q)} - (1-p)\frac{ \big(\mu(1)p+\mu(0)\big)^{H/16} - \big(\mu(1)q+\mu(0)\big)^{H/16}  }{\mu(1) (1-p)(1-q)},
\end{align}
where (i) arises from $(1-p)\mu(1)V_{h+1}^{\star}(1) >0$, (ii) holds by \eqref{eq:basic-facts-finite}.

To control the second term, we first recall that
\begin{align}
    p = 1 - \frac{1}{H} + \frac{c\varepsilon}{H^2}
    \qquad \text{and} \qquad
    q = 1 - \frac{1}{H} - \frac{c\varepsilon}{H^2}.
\end{align}
Then, applying Taylor's theorem to function $f(x) = x^{H/16}$ leads to
\begin{align}
    \big(\mu(1)p+\mu(0)\big)^{H/16} \leq \left(\mu(1)\left(1-\frac{1}{H}\right)+\mu(0)\right)^{H/16} + \frac{c\varepsilon}{H^2}\frac{H}{16}\big(\mu(1)p+\mu(0)\big)^{H/16 -1} \\
    \big(\mu(1)q+\mu(0)\big)^{H/16} \leq \left(\mu(1)\left(1-\frac{1}{H}\right)+\mu(0)\right)^{H/16} - \frac{c\varepsilon}{H^2}\frac{H}{16}\big(\mu(1)p+\mu(0)\big)^{H/16 -1} \\
\end{align}

\subsection{Proof of Theorem~\ref{thm:infinite-lwoer-bound}}
\paragraph{Construction of the hard instances.}
Consider the following two MDPs $\left\{ \mathcal{M}_{\theta} = (\mathcal{S}, \mathcal{A}, P_{\theta}, r, \gamma)\right\}$,
where $\cS = \{0, 1, \ldots, S-1\}$, $\mathcal{A} = \{0, 1\}$, and $\theta \in \{0, 1\}$.  Suppose that $H\geq 32$ and there exist a constant $C>0$. We also find it convenient to introduce the following state distribution:
\begin{align}\label{infinite-mu-assumption}
       \mu(s) = \frac{1}{CS}\mathds{1}(s = 0) + \Big(1 - \frac{1}{CS}\Big)\mathds{1}(s = 1), \qquad \text{where } \frac{1}{CS} \leq \frac{1}{4 \gamma}.
\end{align}
With this distribution in hand, we define the transition kernel $P_{\theta}$ of the MDP $\mathcal{M}_\theta$ as follows:
Define the transition matrix as
\begin{align*}
P_\theta(s^{\prime} \mymid s, a) = \left\{ \begin{array}{lll}
         p\mathds{1}(s^{\prime} = 0) + (1-p)\mu(s^{\prime}) & \text{for} & (s, a) = (0, \theta) \\
         q\mathds{1}(s^{\prime} = 0) + (1-q)\mu(s^{\prime}) & \text{for} & (s, a) = (0, 1-\theta) \\
         \mathds{1}(s^{\prime} = s) & \text{for}   & (s, a) = (1, 0) \\ 
         (2\gamma-1)\mathds{1}(s^{\prime} = s) + 2(1-\gamma)\mu(s^{\prime}) & \text{for}   & (s, a) = (1, 1) \\ 
         \gamma\mathds{1}(s^{\prime} = s) + (1-\gamma)\mu(s^{\prime}) & \text{for}   & s > 1 \
                \end{array}\right.
\end{align*}
where $p$ and $q$ are defined to be 
\begin{align}
p = \gamma + \frac{9(1-\gamma)^2\varepsilon}{\gamma},\qquad q = \gamma - \frac{9(1-\gamma)^2\varepsilon}{\gamma}.
\end{align} 
In addition, the reward function for any MDP $\mathcal{M}_\theta$ is defined as 
\begin{align*}
r(s, a) = \left\{ \begin{array}{lll}
         1 & \text{for} & s = 0 \\
         \frac{1}{2} & \text{for}   & (s, a) = (1, 0) \\ 
         0 & \text{for}   & (s, a) = (1, 1) \\ 
         0 & \text{for}   & s > 1 \
                \end{array}\right.
\end{align*}
% Then it is obvious that $\mu_{\mathsf{b}}(s, a) = \mu(s)\pi_{\mathsf{b}}(a \mymid s)$.
% We let $\rho(s) = \ind(s = 0)$.

\paragraph{Construction of the batch dataset.}
To proceed, we generate a batch dataset with the following initial state distribution $\rhob$ and behavior policy $\pib$: 
\begin{align*}
    \rhob (s) = \mu(s)\quad \text{and } \quad \pi^{\mathsf{b}}(a \mymid s) = \frac{1}{2} \qquad \forall (s,a,h)\in \cS\times \cA,
\end{align*}
where $\mu$ has been defined in \eqref{infinite-mu-assumption}. 
As a result, we can define and calculate the visiting distribution of the behavior policy $\pib$ by applying a little algebra:
\begin{align}
\myrho(s) &= d^{\pib}(s; \rhob) \coloneqq (1-\gamma) \mathbb{E}\left[\sum_{t=0}^\infty \gamma^t \mathbb{P}\big(s_t=s\mid s_{0}\sim \rhob;\pib\big)\right] = \mu(s), \qquad \forall s\in\cS,
\end{align}
which directly implies that
\begin{align}
\myrho(s, a) &= d^{\pib}(s,a; \rhob) \coloneqq \mathbb{E}\left[\sum_{t=0}^\infty \gamma^t \mathbb{P}\big(s_t=s, a_t = a\mid s_{0}\sim \rhob;\pib\big)\right]\\
& = \myrho(s)\pi^{\mathsf{b}}(a \mymid s) =  \mu(s)\pi^{\mathsf{b}}(a \mymid s), \qquad \forall (s,a)\in\cS\times \cA.
\end{align}

With above definitions, now we are ready to derive the lower bound.
\paragraph{Useful facts of hard MDPs.}
We set the goal as learning  a $\varepsilon$-optimal policy with a specific initial state distribution $\rho(s) = \ind(s = 0)$ w.r.t a particular MDP $\mathcal{M}_\theta$, i.e.,
\begin{align} \label{eq:infinite-lower-goal}
      \big\langle \rho, V_\theta^{ \star} - V_\theta^{\pi} \big\rangle \ge \varepsilon.
\end{align}
To begin with, for any policy $\pi$, it is observed that the value of state $s=0$ is
\begin{align}
    V_\theta^\pi(0) &= \mathbb{E}_\pi[1 + \gamma P_{s, \pi(s)}] \nonumber \\
    & = 1 + \gamma \pi(\theta \mymid 0) \big[ \big(p + (1-p)\mu(0)\big) V_\theta^\pi(0) + (1-p) \mu(1) V_\theta^\pi(1)\big] \nonumber \\
    & \qquad + \gamma \pi(1-\theta \mymid 0) \big[\big(q + (1-q) \mu(0)\big) V_\theta^\pi(0) + (1-q)\mu(1) V_\theta^\pi(1)\big] \nonumber \\
   & = 1 + \gamma\left[p \pi(\theta \mymid 0) + q \pi(1-\theta \mymid0) + \mu(0) - p \pi(\theta \mymid 0) \mu(0) - q \pi(1-\theta \mymid0)\mu(0) \right]V_\theta^{\pi}(0) \nonumber\\
&\qquad + \gamma \mu(1) \left[ 1 - p\pi(\theta \mymid 0)  -q \pi(1-\theta\mymid 0)\right]V_\theta^{\pi}(1) \nonumber\\
& \overset{\mathrm{(i)}}{=} 1 + \gamma \left[ x_\pi + (1- x_\pi)\mu(0) V_\theta^{\pi}(0) +  (1 - x_\pi) \mu(1) V_\theta^{\pi}(1)\right]  \nonumber\\
& =  1 + \gamma \big[ \big(\mu(1)x_\pi +\mu(0)\big) V_\theta^{\pi}(0) + (1-x_\pi)\mu(1)V_\theta^{\pi}(1) \big], \label{eq:infinite-Value-0}
\end{align}
where (i) holds by letting 
\begin{align}
x_\pi = p\pi(\theta\mymid 0) + q\pi(1-\theta\mymid 0).\label{eq:infinite-x-h}
\end{align}
Rearranging \eqref{eq:infinite-Value-0} directly yields
\begin{align}\label{eq:infinite-value-0-expression}
    V_\theta^\pi(0)= \frac{1 + \gamma(1-x_\pi)\mu(1)V_\theta^{\pi}(1)}{1 - \gamma\big(\mu(1)x_\pi +\mu(0)\big)}.
\end{align}

Additionally,  the value of state $s=1$ obeys

\begin{align*}
        V_\theta^{\pi}(1) &= \pi(0 \mymid 1) \left( \frac{1}{2} + \gamma V_\theta^{\pi}(1)\right) + \pi(1 \mymid 1) \gamma \left[ \left(1- \frac{2(1-\gamma)}{CS}\right)V_\theta^{\pi}(1) + \frac{2(1-\gamma)}{CS}V_\theta^{\pi}(0)\right]\\
        & \overset{\mathrm{(i)}}{\leq} \pi(0 \mymid 1) \left( \frac{1}{2} + \gamma V_\theta^{\pi}(1)\right) + \pi(1 \mymid 1) \gamma \left[ \left(1- \frac{2(1-\gamma)}{CS}\right)V_\theta^{\pi}(1) + \frac{2(1-\gamma)}{CS}\frac{1}{1-\gamma}\right]\\
        & \overset{\mathrm{(ii)}}{\leq} \pi(0 \mymid 1) \left( \frac{1}{2} + \gamma V_\theta^{\pi}(1)\right) + \pi(1 \mymid 1) \left[ \frac{1}{2} + \gamma \left(1- \frac{2(1-\gamma)}{CS}\right)V_\theta^{\pi}(1) \right]\\
        & = \frac{1}{2} + \gamma V_\theta^{\pi}(1) - \frac{2\gamma(1-\gamma)}{CS} V_\theta^{\pi}(1) \pi(1 \mymid 1)
\end{align*}
where (i) arises from the trivial facts $ 0\leq V_\theta^{\pi}(s) \leq \frac{1}{1-\gamma}$ for any policy $\pi$ and all $s\in\cS $, and (ii) holds from \eqref{infinite-mu-assumption}.
The above result implies that the optimal policy $\pi_\theta^\star(1) = 0$, which leads to
\begin{align}\label{eq:infinite-value-1-star}
        V_\theta^{\pi}(1) &\le V_\theta^{\star}(1) = \frac{1}{2(1-\gamma)}.
\end{align}

% With the above MDPs, we observe that for any policy $\pi$ and $\mu(0) \le \frac{1}{2}$, we have
% \begin{align*}
% V^{\pi}(0) &= \mathbb{E}_{\pi} \Big[1 + \gamma\Big(\big(\mu(1)x+\mu(0)\big) V^{\pi}(0) + (1-x)\mu(1)V^{\pi}(1)\Big) \Big], \\
% V^{\pi}(1) &\le V^{\star}(1) = \frac{1}{2(1-\gamma)},
% \end{align*}
% where $x = p\pi(\theta\mymid 0) + q\pi(1-\theta\mymid 0)$.
It is easily verified that the optimal policy for $\mathcal{M}_\theta$ at state $0$ is $\pi_\theta^\star(0) = \theta$. Now we are ready to control \eqref{eq:infinite-lower-goal} as follows:
\begin{align}
    \langle \rho, V_\theta^{\star} - V_\theta^{\pi}\rangle &= V_\theta^{\star}(0) - V_\theta^{\pi}(0) \nonumber \\
    & \overset{\mathrm{(i)}}{=} \frac{1 + \gamma(1-p)\mu(1)V_\theta^{\star}(1)}{1 - \gamma\big(\mu(1)p +\mu(0)\big)} - \frac{1 + \gamma(1-x_\pi)\mu(1)V_\theta^{\pi}(1)}{1 - \gamma\big(\mu(1)x_\pi +\mu(0)\big)} \nonumber  \\
    & \overset{\mathrm{(ii)}}{\geq} \frac{1 + \gamma(1-p)\mu(1)V_\theta^{\star}(1)}{1 - \gamma\big(\mu(1)p +\mu(0)\big)} - \frac{1 + \gamma(1-x_\pi)\mu(1)V_\theta^{\star}(1)}{1 - \gamma\big(\mu(1)x_\pi +\mu(0)\big)}\\
    & = \frac{}{}
\end{align}
where (i) holds from applying \eqref{eq:infinite-value-0-expression} and we obtain the last inequality if the following fact holds
\begin{align}\label{eq:infinite-delta-key-auxiliary}
    \frac{1 + \gamma(1-p)\mu(1)V_\theta^{\star}(1)}{1 - \gamma\big(\mu(1)p +\mu(0)\big)} - \frac{1 + \gamma(1-x_\pi)\mu(1)V_\theta^{\star}(1)}{1 - \gamma\big(\mu(1)x_\pi +\mu(0)\big)} \geq
\end{align}

\paragraph{Deriving the lower bound.}

Then
\begin{align*}
V^{\star}(0) - V^{\pi}(0) \ge \frac{1 + \gamma\mu(1)(1-p)V^{\star}(1)}{1 - \gamma\big(\mu(1)p + \mu(0)\big)} - \frac{1 + \gamma\mu(1)(1-x)V^{\star}(1)}{1 - \gamma\big(\mu(1)x + \mu(0)\big)},
\end{align*}
which implies, if $|\pi(0) - \pi^{\star}(0)| \ge \frac{1}{2}$, 
\begin{align*}
\langle \rho, V^{\star} - V^{\pi}\rangle = V^{\star}(0) - V^{\pi}(0) \ge \varepsilon.
\end{align*}

In addition,
\begin{align*}
\mathsf{KL}(p \parallel q) = p\log \frac{p}{q} + (1-p)\log \frac{1-p}{1-q} \asymp (1-\gamma)^3\varepsilon^2.
\end{align*}
Then Fano's inequality gives \lxs{Need Le Cam}
\begin{align*}
\inf_{\pi}\sup_{\mathcal{M}_{\theta}} \mathbb{P}\big(\langle \rho, V^{\star} - V^{\pi}\rangle \ge \varepsilon\big) \ge \frac{1}{5},
\end{align*}
since there are $O\left(\frac{1}{(1-\gamma)^3\varepsilon^2}\right)$ samples for $s = 0$,
provided that
\begin{align*}
N \lesssim \frac{CS}{(1-\gamma)^3\varepsilon^2},
\end{align*}
Notice that for $\pi^{\star}(0) = \theta$, we have 
\begin{align*}
d^{\star}(0, \theta) \ge (1-\gamma)\sum_{k \ge 0}\rho(0)\gamma^k\mathbb{P}_{\theta}^k(0 \mymid 0, \theta) \ge (1-\gamma)\sum_{k \ge 0}\rho(0)\gamma^{2k} \ge \frac{1}{1+\gamma}.
\end{align*}
Hence, one can check that $\Cstar = \frac{2}{S\mu(0)} = 2C$, and the lower bound is ready.

\paragraph{Proof of inequality \eqref{eq:infinite-delta-key-auxiliary}.}
We express the term of interest out
\begin{align}
    &\frac{1 + \gamma(1-p)\mu(1)V_\theta^{\star}(1)}{1 - \gamma\big(\mu(1)p +\mu(0)\big)} - \frac{1 + \gamma(1-x_\pi)\mu(1)V_\theta^{\star}(1)}{1 - \gamma\big(\mu(1)x_\pi +\mu(0)\big)} \nonumber \\
    &=  \frac{\big[1 - \gamma\big(\mu(1)x_\pi +\mu(0)\big)\big]\big[1 + \gamma(1-p)\mu(1)V_\theta^{\star}(1)\big] - \big[1 - \gamma\big(\mu(1)p +\mu(0)\big)\big]\big[1 + \gamma(1-x_\pi)\mu(1)V_\theta^{\star}(1)\big]}{ \underbrace{\left[1 - \gamma\big(\mu(1)p +\mu(0)\big)\right]\left[1 - \gamma\big(\mu(1)x_\pi +\mu(0)\big)\right] }_{\eqqcolon A}} \nonumber \\
    & = \frac{1}{A}\Big[\gamma \mu(1) (p-x_\pi) + \gamma \mu(1)V_\theta^{\star}(1) \Big((x_\pi-p) + \gamma\big(\mu(1)p +\mu(0)\big)(1-x_\pi) - \gamma \big(\mu(1)x_\pi +\mu(0)\big) (1-p)\Big)\Big] \nonumber \\
    & = \frac{\gamma \mu(1) (p-x_\pi)}{A}\Big[1-(1-\gamma)V_\theta^{\star}(1)\Big] \nonumber \\
    & \overset{\mathrm{(i)}}{=}  \frac{\gamma \mu(1) (p-x_\pi)}{2A}
\end{align}
where (i) arises from the fact in \eqref{eq:infinite-value-1-star}.

The remainder of the proof is to further control the denominator $A$. Plugging in the definitions of $p$ and $x_\pi$ (see \eqref{eq:infinite-x-h}), we arrive at
\begin{align}
    A = 
\end{align}
